# Supplementary material for: Cosmology from the two-dimensional renormalization group acting as the Ricci flow
Source: arXiv:1909.01374 source file (2020-05-11)
Supplement: Supplementary file 1 [file Calculations_for_Cosmology_I.pdf]

# Calculations for *Cosmology* . . .

Daniel Friedan

*New High Energy Theory Center and Department of Physics and Astronomy,  
Rutgers, The State University of New Jersey,  
Piscataway, New Jersey 08854-8019 U.S.A. and*

*Science Institute, The University of Iceland, Reykjavik, Iceland*

dfriedan@gmail.com      www.physics.rutgers.edu/~friedan/

September 3, 2019

This note shows calculations for the paper *Cosmology from the two-dimensional renormalization group acting as the Ricci flow*. Numerical calculations are performed in the accompanying SageMath notebooks. Sections here that contain numerical results from the notebooks are labeled **SNB**. The section numbering in the notebooks follows the numbering here.

To run the notebooks, either install SageMath from [sagemath.org](http://sagemath.org) or create an account at [cocalc.com](http://cocalc.com) and upload the notebooks to run there. SageMath is a free open-source mathematics software system. Both free and paid accounts are available at [cocalc.com](http://cocalc.com). Paying for an account supports SageMath (see [reasons-for-purchasing-a-subscription](#)). Open-source mathematics software such as SageMath is essential for scientific research. Scientific results must be completely open to scrutiny. Closed-source mathematics software blocks scrutiny.

## Contents

|          |                                                                               |          |
|----------|-------------------------------------------------------------------------------|----------|
| <b>1</b> | <b>SO(<math>d</math>)-invariant geometry on <math>I \times S^{d-1}</math></b> | <b>3</b> |
| 1.1      | $I \times S^{d-1} \subset \mathbb{R}^d$                                       | 3        |
| 1.2      | $g_{\mu\nu}$ in conformally flat gauge                                        | 3        |
| 1.3      | $R_{\mu\nu}$                                                                  | 4        |
| 1.4      | $\nabla_\mu v_\nu + \nabla_\nu v_\mu$                                         | 4        |
| <b>2</b> | <b><math>R_{\mu\nu} = \nabla_\mu v_\nu + \nabla_\nu v_\mu</math> as ode</b>   | <b>5</b> |
| <b>3</b> | <b>Analytically continue to real time</b>                                     | <b>5</b> |
| <b>4</b> | <b><math>T_{\mu\nu}</math></b>                                                | <b>5</b> |
| <b>5</b> | <b>The constant of motion <math>C</math></b>                                  | <b>6</b> |
| <b>6</b> | <b>The <math>C = 0</math> cosmological solution</b>                           | <b>7</b> |
| <b>7</b> | <b>The cosmological parameters [SNB I-1]</b>                                  | <b>8</b> |
| 7.1      | Formulas for $H$ , $q$ , $w$ , and $\Omega$                                   | 8        |
| 7.2      | Estimate $t_0$ and $t'_0$                                                     | 9        |
| 7.3      | The limit $t \rightarrow 0$                                                   | 10       |
| 7.4      | The limit $t \rightarrow t_{\max}$                                            | 10       |
| 7.5      | Table of parameters for selected $z$ values                                   | 10       |
| 7.6      | Plot the cosmological parameters                                              | 11       |

|           |                                                                              |    |
|-----------|------------------------------------------------------------------------------|----|
| 7.7       | Plot the conformal diagram                                                   | 11 |
| <b>8</b>  | <b>Analysis of the real-time ode continued</b>                               | 12 |
| 8.1       | Real-time phase portrait [SNB I-1]                                           | 12 |
| 8.2       | Asymptotic behavior of the $C \neq 0$ solutions                              | 13 |
| 8.3       | Non-analyticity of $C \neq 0$ solutions                                      | 13 |
| 8.4       | Asymptotic behavior of the separatrices $S, S'$ [SNB I-1]                    | 14 |
| 8.5       | Numerical calculation of the invariant $c_S$ [SNB I-2]                       | 14 |
| <b>9</b>  | <b>Euclidean signature phase portrait [SNB I-3]</b>                          | 17 |
| <b>10</b> | <b><math>v_\mu = \partial_\mu \chi \iff \chi</math> is the dilaton field</b> | 18 |

# 1 $\mathbf{SO}(d)$ -invariant geometry on $I \times S^{d-1}$

We are investigating the fixed-point equation

$$R_{\mu\nu} = \nabla_\mu v_\nu + \nabla_\nu v_\mu \quad (1.1)$$

for a Riemannian metric  $g_{\mu\nu}$  and a vector field  $v^\mu$  on  $I \times S^3$  both invariant under  $\mathbf{SO}(4)$ .

## 1.1 $I \times S^{d-1} \subset \mathbb{R}^d$

Consider  $I \times S^{d-1}$  as a spherical shell in  $\mathbb{R}^d$  with coordinates  $x^\mu$ . The euclidean metric is

$$\delta_{\mu\nu} dx^\mu dx^\nu = dr^2 + r^2 ds_{S^3}^2 = r^2(d\tau^2 + ds_{S^3}^2) \quad r = \sqrt{\delta_{\mu\nu} x^\mu x^\nu} \quad r = e^\tau \quad (1.2)$$

where  $ds_{S^{d-1}}^2$  is the  $\mathbf{SO}(d)$ -invariant metric on the unit  $(d-1)$ -sphere.

$$\begin{aligned} \hat{x}^\mu &= r^{-1} x^\mu & \partial_\mu r &= \hat{x}_\mu & dr &= \hat{x}_\mu dx^\mu \\ P_{\mu\nu} &= \delta_{\mu\nu} - \hat{x}_\mu \hat{x}_\nu & \partial_\mu \hat{x}_\nu &= r^{-1} P_{\mu\nu} & \partial_\mu (r^{-1} \hat{x}_\nu) &= r^{-2} (P_{\mu\nu} - \hat{x}_\mu \hat{x}_\nu) \\ \partial_\tau &= x^\mu \partial_\mu & d\tau &= r^{-1} \hat{x}_\mu dx^\mu & \partial_\mu \tau &= r^{-1} \hat{x}_\mu \\ \partial_\alpha &= r^{-1} \hat{x}_\alpha \partial_\tau & \text{on invariant functions} & & & \\ r^{-2} \delta_{\mu\nu} dx^\mu dx^\nu &= d\tau^2 + ds_{S^{d-1}}^2 & d\tau^2 &= r^{-2} \hat{x}_\mu \hat{x}_\nu dx^\mu dx^\nu & ds_{S^{d-1}}^2 &= r^{-2} P_{\mu\nu} dx^\mu dx^\nu \end{aligned} \quad (1.3)$$

## 1.2 $g_{\mu\nu}$ in conformally flat gauge

The general  $\mathbf{SO}(d)$ -invariant metric is

$$g_{\mu\nu}(x) dx^\mu dx^\nu = F_1(r)^2 dr^2 + F_2(r)^2 ds_{S^{d-1}}^2 \quad (1.4)$$

After a suitable reparametrization  $r \rightarrow \tau(r)$  the metric is conformally flat

$$\begin{aligned} g_{\mu\nu} dx^\mu dx^\nu &= e^{2f(\tau)} (d\tau^2 + ds_{S^{d-1}}^2) \\ \frac{dr}{d\tau} &= \frac{F_2}{F_1} & F_2(r) &= e^{f(\tau)} \\ g_{\mu\nu} &= e^{2f(\tau)} r^{-2} \delta_{\mu\nu} = e^{2\tilde{f}(\tau)} \delta_{\mu\nu} & \tilde{f}(\tau) &= f(\tau) - \tau \end{aligned} \quad (1.5)$$

Define

$$f_\tau = \partial_\tau f \quad (1.6)$$

so

$$\partial_\mu \tilde{f} = r^{-1} \hat{x}_\mu \partial_\tau \tilde{f} \quad \partial_\tau \tilde{f} = f_\tau - 1 \quad (1.7)$$

The covariant derivative is

$$\begin{aligned} \nabla_\nu w_\mu &= \partial_\nu w_\mu - \Gamma_{\mu\nu}^\alpha w_\alpha \\ \Gamma_{\mu\nu}^\alpha &= \delta_\mu^\alpha \partial_\nu \tilde{f} + \delta_\nu^\alpha \partial_\mu \tilde{f} - \delta_{\mu\nu} \partial^\alpha \tilde{f} = r^{-1} (\delta_\mu^\alpha \hat{x}_\nu + \delta_\nu^\alpha \hat{x}_\mu - \delta_{\mu\nu} \hat{x}^\alpha) \partial_\tau \tilde{f} \end{aligned} \quad (1.8)$$

### 1.3 $R_{\mu\nu}$

The curvature tensor is

$$R_{\mu\beta\nu}^{\alpha} = \partial_{\beta}\Gamma_{\mu\nu}^{\alpha} + \Gamma_{\sigma\beta}^{\alpha}\Gamma_{\mu\nu}^{\sigma} - \Gamma_{\nu\beta}^{\sigma}\Gamma_{\mu\sigma}^{\alpha} - (\beta \leftrightarrow \nu) \quad (1.9)$$

The Ricci tensor is

$$\begin{aligned} R_{\mu\nu} &= R_{\mu\alpha\nu}^{\alpha} = -\delta_{\mu\nu}\partial_{\alpha}\partial^{\alpha}\tilde{f} + (d-2)\left(-\partial_{\mu}\partial_{\nu}\tilde{f} + \partial_{\mu}\tilde{f}\partial_{\nu}\tilde{f} - \delta_{\mu\nu}\partial^{\alpha}\tilde{f}\partial_{\alpha}\tilde{f}\right) \\ &= -(d-1)\partial_{\tau}f_{\tau}r^{-2}\hat{x}_{\mu}\hat{x}_{\nu} - [\partial_{\tau}f_{\tau} + (d-2)(f_{\tau}^2 - 1)]r^{-2}P_{\mu\nu} \\ R_{\mu\nu}dx^{\mu}dx^{\nu} &= -(d-1)\partial_{\tau}f_{\tau}d\tau^2 - [\partial_{\tau}f_{\tau} + (d-2)(f_{\tau}^2 - 1)]ds_{S^{d-1}}^2 \end{aligned} \quad (1.10)$$

The scalar curvature is

$$R = g^{\mu\nu}R_{\mu\nu} = e^{-2f}r^2\delta^{\mu\nu}R_{\mu\nu} = -e^{-2f}(d-1)[2\partial_{\tau}f_{\tau} + (d-2)(f_{\tau}^2 - 1)] \quad (1.11)$$

The Einstein tensor is

$$\begin{aligned} G_{\mu\nu} &= R_{\mu\nu} - \frac{1}{2}Rg_{\mu\nu} \\ G_{\mu\nu}dx^{\mu}dx^{\nu} &= \frac{1}{2}(d-2)(d-1)(f_{\tau}^2 - 1)d\tau^2 \\ &\quad + \frac{1}{2}(d-2)[2\partial_{\tau}f_{\tau} + (d-3)(f_{\tau}^2 - 1)]ds_{S^3}^2 \end{aligned} \quad (1.12)$$

In  $d = 4$  dimensions

$$\begin{aligned} R_{\mu\nu}dx^{\mu}dx^{\nu} &= -3\partial_{\tau}f_{\tau}d\tau^2 - (\partial_{\tau}f_{\tau} + 2f_{\tau}^2 - 2)ds_{S^3}^2 \\ R &= -e^{-2f}6(\partial_{\tau}f_{\tau} + f_{\tau}^2 - 1) \\ G_{\mu\nu}dx^{\mu}dx^{\nu} &= 3(f_{\tau}^2 - 1)d\tau^2 + (2\partial_{\tau}f_{\tau} + f_{\tau}^2 - 1)ds_{S^3}^2 \end{aligned} \quad (1.13)$$

### 1.4 $\nabla_{\mu}v_{\nu} + \nabla_{\nu}v_{\mu}$

The general  $\mathbf{SO}(d)$ -invariant vector field  $v = v^{\mu}(x)\partial_{\mu}$  is

$$\begin{aligned} v^{\mu}\partial_{\mu} &= v^{\tau}(\tau)\partial_{\tau} & v^{\mu} &= v^{\tau}x^{\mu} \\ v_{\mu}dx^{\mu} &= v_{\tau}d\tau & v_{\tau} &= g_{\tau\tau}v^{\tau} = e^{2f}v^{\tau} & v_{\mu} &= v_{\tau}r^{-1}\hat{x}_{\mu} \end{aligned} \quad (1.14)$$

Its covariant derivative is

$$\nabla_{\mu}v_{\nu} = \partial_{\mu}v_{\nu} - \Gamma_{\mu\nu}^{\alpha}v_{\alpha} = (\partial_{\tau}v_{\tau} - f_{\tau}v_{\tau})r^{-2}\hat{x}_{\mu}\hat{x}_{\nu} + f_{\tau}v_{\tau}r^{-2}P_{\mu\nu} \quad (1.15)$$

so

$$\begin{aligned} (\nabla_{\mu}v_{\nu} + \nabla_{\nu}v_{\mu})dx^{\mu}dx^{\nu} &= (2\partial_{\tau}v_{\tau} - 2f_{\tau}v_{\tau})d\tau^2 + 2f_{\tau}v_{\tau}ds_{S^{d-1}}^2 \\ 2\nabla_{\sigma}v^{\sigma} &= 2a^{-2}[\partial_{\tau}v_{\tau} + (d-2)f_{\tau}v_{\tau}] \\ (\nabla_{\mu}v_{\nu} + \nabla_{\nu}v_{\mu} - \nabla_{\sigma}v^{\sigma}g_{\mu\nu})dx^{\mu}dx^{\nu} &= (\partial_{\tau}v_{\tau} - df_{\tau}v_{\tau})d\tau^2 \\ &\quad - (\partial_{\tau}v_{\tau} + (d-4)f_{\tau}v_{\tau})ds_{S^{d-1}}^2 \end{aligned} \quad (1.16)$$

In  $d = 4$  dimensions

$$(\nabla_{\mu}v_{\nu} + \nabla_{\nu}v_{\mu} - \nabla_{\sigma}v^{\sigma}g_{\mu\nu})dx^{\mu}dx^{\nu} = (\partial_{\tau}v_{\tau} - 4f_{\tau}v_{\tau})d\tau^2 - (\partial_{\tau}v_{\tau})ds_{S^3}^2 \quad (1.17)$$

## 2 $R_{\mu\nu} = \nabla_\mu v_\nu + \nabla_\nu v_\mu$ as ode

The fixed point equation  $R_{\mu\nu} = \nabla_\mu v_\nu + \nabla_\nu v_\mu$  is equivalent to

$$G_{\mu\nu} = R_{\mu\nu} - \frac{1}{2}Rg_{\mu\nu} = \nabla_\mu v_\nu + \nabla_\nu v_\mu - \nabla_\sigma v^\sigma g_{\mu\nu} \quad (2.1)$$

In the invariant case, using (1.12) and (1.16), this is

$$\begin{aligned} \frac{1}{2}(d-2)(d-1)(f_\tau^2 - 1) &= \partial_\tau v_\tau - df_\tau v_\tau \\ (d-2)\partial_\tau f_\tau + \frac{1}{2}(d-2)(d-3)(f_\tau^2 - 1) &= -\partial_\tau v_\tau - (d-4)f_\tau v_\tau \end{aligned} \quad (2.2)$$

In  $d = 4$  dimensions

$$\begin{aligned} 3(f_\tau^2 - 1) &= \partial_\tau v_\tau - 4f_\tau v_\tau \\ 2\partial_\tau f_\tau + (f_\tau^2 - 1) &= -\partial_\tau v_\tau \end{aligned} \quad (2.3)$$

which is the ordinary differential equation

$$\partial_\tau f_\tau = -2f_\tau v_\tau - 2f_\tau^2 + 2 \quad \partial_\tau v_\tau = 4f_\tau v_\tau + 3f_\tau^2 - 3 \quad (2.4)$$

## 3 Analytically continue to real time

Analytically continue from conformal euclidean time  $\tau$  to conformal real time  $T$

$$\begin{aligned} e^{2f}(d\tau^2 + ds_{S^{d-1}}^2) &= e^{2f}(-dT^2 + ds_{S^{d-1}}^2) \\ \tau = iT \quad d\tau = i dT \quad \partial_\tau &= i^{-1}\partial_T \\ df = f_\tau d\tau = f_T dT \quad f_\tau &= i^{-1}f_T \quad v_\tau d\tau = v_T dT \quad v_\tau = i^{-1}v_T \end{aligned} \quad (3.1)$$

In co-moving time  $t$

$$\begin{aligned} e^{2f}(-dT^2 + ds_{S^{d-1}}^2) &= -dt^2 + a^2 ds_{S^{d-1}}^2 \\ dt = e^f dT \quad a = e^f \quad \partial_t &= a^{-1}\partial_T \quad \partial_t a = a^{-1}\partial_T a = f_T \end{aligned} \quad (3.2)$$

The Hubble parameter  $H$  and the deceleration parameter  $q$  are

$$H = a^{-1}\partial_t a = a^{-1}f_T \quad q = -\frac{a\partial_t^2 a}{(\partial_t a)^2} = -\frac{\partial_T f_T}{f_T^2} \quad (3.3)$$

The ode (2.4) becomes in real time

$$\partial_T f_T = -2f_T v_T - 2f_T^2 - 2 \quad \partial_T v_T = 4f_T v_T + 3f_T^2 + 3 \quad (3.4)$$

## 4 $T_{\mu\nu}$

The fixed point equation  $R_{\mu\nu} = \nabla_\mu v_\nu + \nabla_\nu v_\mu$  is equivalent to Einstein's equation

$$G_{\mu\nu} = R_{\mu\nu} - \frac{1}{2}Rg_{\mu\nu} = 8\pi G T_{\mu\nu} \quad (4.1)$$

with energy-momentum tensor

$$T_{\mu\nu} = \frac{1}{8\pi G} (\nabla_\mu v_\nu + \nabla_\nu v_\mu - g_{\mu\nu} \nabla^\alpha v_\alpha) \quad (4.2)$$

given in the invariant case by (1.16)

$$T_{\mu\nu} dx^\mu dx^\nu = \frac{1}{8\pi G} [(\partial_T v_T - 4f_T v_T) dT^2 + (\partial_T v_T) ds_{S^{d-1}}^2] \quad (4.3)$$

This is the energy-momentum tensor of a perfect fluid of density  $\rho$  and pressure  $p$

$$\begin{aligned} T_{\mu\nu} dx^\mu dx^\nu &= a^2 (\rho dT^2 + p ds_{S^3}^2) = \rho dt^2 + p a^2 ds_{S^3}^2 \\ \rho &= \frac{1}{8\pi G a^2} (\partial_T v_T - 4f_T v_T) \quad p = \frac{1}{8\pi G a^2} \partial_T v_T \end{aligned} \quad (4.4)$$

Using the fixed point equation (2.4)

$$\rho = \frac{1}{8\pi G a^2} (3f_T^2 + 3) \quad p = \frac{1}{8\pi G a^2} (4f_T v_T + 3f_T^2 + 3) \quad (4.5)$$

The equation-of-state parameter  $w$  and the density parameter  $\Omega$  are

$$w = \frac{p}{\rho} = 1 + \frac{4}{3} \frac{f_T v_T}{f_T^2 + 1} \quad \Omega = \frac{8\pi G \rho}{3H^2} = 1 + \frac{1}{f_T^2} \quad (4.6)$$

The conservation law  $\nabla^\mu T_{\mu\nu} = 0$  in the invariant case is

$$\begin{aligned} T_{\mu\nu} dx^\mu dx^\nu &= -a^2 \rho d\tau^2 + a^2 p ds_{S^3}^2 \quad T_{\mu\nu} = -a^2 \rho r^{-2} \hat{x}_\mu \hat{x}_\nu + a^2 p r^{-2} P_{\mu\nu} \\ \nabla^\mu T_{\mu\nu} &= a^{-2} \partial_\tau (-a^2 \rho) r^{-1} \hat{x}_\nu + (-a^2 \rho) \nabla^\mu (r^{-2} \hat{x}_\mu \hat{x}_\nu) + a^2 p \nabla^\mu (r^{-2} P_{\mu\nu}) \end{aligned} \quad (4.7)$$

$$\begin{aligned} \nabla^\mu (r^{-2} P_{\mu\nu}) &= -a^{-2} (d-1) f_\tau r^{-1} \hat{x}_\nu \\ \nabla^\mu (r^{-2} \delta_{\mu\nu}) &= -2f_\tau r^{-3} \hat{x}_\nu \\ \nabla^\mu (r^{-2} \hat{x}_\mu \hat{x}_\nu) &= a^{-2} (d-3) f_\tau r^{-1} \hat{x}_\nu \end{aligned} \quad (4.8)$$

$$\begin{aligned} \nabla^\mu T_{\mu\nu} &= a^{-2} r^{-1} \hat{x}_\nu [\partial_\tau (-a^2 \rho) + (d-3) f_\tau (-a^2 \rho) - (d-1) f_\tau a^2 p] \\ &= r^{-1} \hat{x}_\nu [-\partial_\tau \rho - (d-1) f_\tau \rho - (d-1) f_\tau p] \end{aligned} \quad (4.9)$$

So  $\nabla^\mu T_{\mu\nu} = 0$  is

$$\partial_T (a^2 \rho) + (d-3) f_T (a^2 \rho) + (d-1) f_T a^2 p = 0 \quad (4.10)$$

or

$$\partial_T \rho + (d-1) f_T (\rho + p) = 0 \quad (4.11)$$

## 5 The constant of motion $C$

If

$$\nabla_\mu v_\nu - \nabla_\nu v_\mu = 0 \quad (5.1)$$

then  $v^\mu$  is a gradient at least locally

$$v_\mu = \partial_\mu \chi \quad (5.2)$$

In the  $\mathbf{SO}(d)$ -invariant case  $v^\mu$  is always a gradient globally,  $v_\tau(\tau) = \partial_\tau \chi$ .

When  $v^\mu$  is locally a gradient then

$$\begin{aligned} R_{\mu\nu} &= \nabla_\mu v_\nu + \nabla_\nu v_\mu = 2\nabla_\mu \nabla_\nu \chi & R &= 2\nabla_\sigma \nabla^\sigma \chi \\ \nabla^\nu R_{\mu\nu} &= 2\nabla_\mu \nabla^\nu \nabla_\nu \chi + 2R_{\sigma\mu} \nabla^\sigma \chi = \nabla_\mu (2\nabla^\nu \nabla_\nu \chi + 2\nabla_\sigma \chi \nabla^\sigma \chi) \\ 0 &= \nabla^\nu \left( R_{\mu\nu} - \frac{1}{2} g_{\mu\nu} R \right) = \nabla_\mu (\nabla_\sigma \nabla^\sigma \chi + 2\nabla_\sigma \chi \nabla^\sigma \chi) = \nabla_\mu (\nabla_\sigma v^\sigma + 2v_\sigma v^\sigma) \end{aligned} \quad (5.3)$$

so there is a constant of motion

$$C' = \nabla_\sigma v^\sigma + 2v_\sigma v^\sigma = R + 4v_\sigma v^\sigma \quad \nabla_\mu C' = 0 \quad (5.4)$$

For convenience normalize the constant of motion

$$C = \frac{-2}{(d-1)(d-2)} (\nabla_\sigma v^\sigma + 2v_\sigma v^\sigma) = \frac{-1}{(d-1)(d-2)} (R + 4v_\sigma v^\sigma) \quad (5.5)$$

In the  $\mathbf{SO}(d)$ -invariant case

$$\begin{aligned} R &= -a^{-2}(d-1) [2\partial_\tau f_\tau + (d-2)(f_\tau^2 - 1)] \\ &= -a^{-2}(d-1) [-4f_\tau v_\tau - (d-2)(f_\tau^2 - 1)] \\ v_\sigma v^\sigma &= a^{-2} v_\tau^2 \end{aligned} \quad (5.6)$$

so

$$C = a^{-2} \left( -f_\tau^2 - \frac{4}{d-2} f_\tau v_\tau - \frac{4}{(d-1)(d-2)} v_\tau^2 + 1 \right) \quad (5.7)$$

Continued to real time

$$C = a^{-2} \left( f_T^2 + \frac{4}{d-2} f_T v_T + \frac{4}{(d-1)(d-2)} v_T^2 + 1 \right) \quad (5.8)$$

In  $d = 4$  dimensions

$$C = a^{-2} \left( f_T^2 + 2f_T v_T + \frac{2}{3} v_T^2 + 1 \right) \quad (5.9)$$

## 6 The $C = 0$ cosmological solution

Define

$$h_\pm = f_T + \beta_\pm v_T \quad \beta_\pm = 1 \pm \frac{1}{\sqrt{3}} \quad (6.1)$$

so that

$$a^2 C = h_+ h_- + 1 \quad (6.2)$$

The ode (3.4) is now

$$\partial_T h_\pm = -1 - h_\pm^2 + \lambda_\pm (h_+ h_- + 1) \quad \lambda_\pm = \frac{\beta_\pm}{\beta_\mp} = 2 \pm \sqrt{3} \quad (6.3)$$

When  $C = 0$  the ode (6.3) becomes

$$\partial_T h_\pm = -1 - h_\pm^2 \quad (6.4)$$

which has the solution

$$h_- = \cot T \quad h_+ = -\tan T \quad (6.5)$$

which is unique up to translation and reflection in  $T$ . Changing variables back to

$$f_T = \frac{\sqrt{3}}{2} (\beta_+ h_- - \beta_- h_+) \quad v_T = \frac{\sqrt{3}}{2} (h_+ - h_-) \quad (6.6)$$

the  $C = 0$  solution becomes

$$\begin{aligned} f_T &= \frac{\sqrt{3}+1}{2} \cot T + \frac{\sqrt{3}-1}{2} \tan T = \frac{\cos 2T + \sqrt{3}}{\sin 2T} \\ v_T &= -\frac{\sqrt{3}}{2} \cot T - \frac{\sqrt{3}}{2} \tan T = \frac{-\sqrt{3}}{\sin 2T} \end{aligned} \quad (6.7)$$

Integrating  $\partial_T f = f_T$  with constant of integration  $\ln t'_0$

$$\begin{aligned} f &= \ln t'_0 + (1 + \nu) \ln \sin T - \nu \ln \cos T \quad \nu = \frac{\sqrt{3}-1}{2} \\ a &= e^f = t'_0 \sin^{1+\nu} T \cos^{-\nu} T \end{aligned} \quad (6.8)$$

The co-moving time  $t$  is

$$\begin{aligned} dt &= a dT \quad \frac{t}{t'_0} = \int_0^T a(T') dT' = \frac{1}{2} B_{\sin^2 T} (1 + \nu/2, 1/2 - \nu/2) \\ t \in (0, t_{\max}) \quad \frac{t_{\max}}{t'_0} &= \int_0^{\frac{\pi}{2}} a(T') dT' = \frac{1}{2} B(1 + \nu/2, 1/2 - \nu/2) = 1.470147 \dots \end{aligned} \quad (6.9)$$

where  $B(p, q)$  is the Euler beta function and  $B_x(p, q)$  is the incomplete beta function

$$\begin{aligned} B_x(p, q) &= \int_0^x s^{p-1} (1-s)^{q-1} ds = 2 \int_0^{\sin^2 \theta=x} \sin^{2p-1} \theta \cos^{2q-1} \theta d\theta \\ &= \frac{x^p}{p} F(p, 1-q; p+1; x) \\ B(p, q) &= B_1(p, q) = \frac{\Gamma(p)\Gamma(q)}{\Gamma(p+q)} \end{aligned} \quad (6.10)$$

$F$  in the second line above is the hypergeometric function  ${}_2F_1$ .

## 7 The cosmological parameters [SNB I-1]

### 7.1 Formulas for $H$ , $q$ , $w$ , and $\Omega$

Substituting in (3.3)

$$\begin{aligned} H &= a^{-1} f_T = (t'_0 \sin^{1+\nu} T \cos^{-\nu} T)^{-1} \left( \frac{\cos 2T + \sqrt{3}}{\sin 2T} \right) \\ &= \frac{1}{t'_0} (\sin^{-2-\nu} T \cos^{-1+\nu} T) \frac{1}{2} (\cos 2T + \sqrt{3}) \\ &= \frac{1}{t'_0} (\sin^{-2-\nu} T \cos^{-1+\nu} T) (\cos^2 T + \nu) \end{aligned} \quad (7.1)$$

$$\begin{aligned}
q &= -f_T^{-2} \partial f_T = - \left( \frac{\cos 2T + \sqrt{3}}{\sin 2T} \right)^{-2} \left( \frac{\sqrt{3} + 1}{2} \frac{-1}{\sin^2 T} + \frac{\sqrt{3} - 1}{2} \frac{1}{\cos^2 T} \right) \\
&= \frac{2(1 + \sqrt{3} \cos 2T)}{(\cos 2T + \sqrt{3})^2} = \frac{\sqrt{3} \cos^2 T - \nu}{(\cos^2 T + \nu)^2}
\end{aligned} \tag{7.2}$$

The expansion decelerates ( $q > 0$ ) for  $T < T_{q=0}$  then accelerates ( $q < 0$ ) for  $T_{q=0} < T$ .

$$T_{q=0} = \frac{\arccos(-1/\sqrt{3})}{2} = \frac{\pi - \arccos(1/\sqrt{3})}{2} = \frac{\pi - \arctan(\sqrt{2})}{2} = 0.6959 \frac{\pi}{2} \tag{7.3}$$

Substituting in (7.4) gives formulas for  $w$  and  $\Omega$

$$\begin{aligned}
w &= 1 + \frac{4}{3} \frac{f_T v_T}{f_T^2 + 1} \\
&= 1 + \frac{4}{3} \left( \frac{\cos 2T + \sqrt{3}}{\sin 2T} \right) \left( \frac{-\sqrt{3}}{\sin 2T} \right) \left[ 1 + \left( \frac{\cos 2T + \sqrt{3}}{\sin 2T} \right)^2 \right]^{-1} \\
&= \frac{\cos 2T}{3 \cos 2T + 2\sqrt{3}} \\
\Omega &= 1 + \frac{1}{f_T^2} = 1 + \left( \frac{\sin 2T}{\cos 2T + \sqrt{3}} \right)^2
\end{aligned} \tag{7.4}$$

## 7.2 Estimate $t_0$ and $t'_0$

Use  $q_0 = -0.60$  as the present value of the deceleration parameter. Solve  $q(T_0) = q_0$  numerically to estimate the present conformal time

$$T_0 = 0.77 \frac{\pi}{2} \tag{7.5}$$

Then calculate the present value of the Hubble parameter by substituting  $T_0$  in (7.1) to fix  $t'_0$  in units of the Hubble time  $t_H = H_0^{-1}$

$$t'_0 = (\sin^{-2-\nu} T_0 \cos^{-1+\nu} T_0) (\cos^2 T_0 + \nu) t_H = 1.1 t_H \tag{7.6}$$

The Hubble time is

$$t_H = 4.55 \times 10^{17} \text{s} = 1.44 \times 10^{10} \text{y} \tag{7.7}$$

Now  $t_0$ ,  $t_{\max}$ , and the present values  $a_0$ ,  $w_0$ , and  $\Omega_0$  can be calculated from (6.9), (6.8), and (7.4)

$$t_0 = 0.73 t_H \quad t_{\max} = 1.6 t_H \quad a_0 = 1.5 t_H \quad w_0 = -0.61 \quad \Omega_0 = 1.5 \tag{7.8}$$

Once  $a_0$  is estimated, the redshift can be calculated

$$z = \frac{a_0}{a} - 1 \tag{7.9}$$

In particular,  $q = 0$  at  $z = 0.18$  and  $T = \frac{1}{2}T_0$  at  $z = 1.69$ .

### 7.3 The limit $t \rightarrow 0$

In the limit  $T \rightarrow 0$

$$\begin{aligned}
f_T &\rightarrow \frac{1+\nu}{T} & v_T &\rightarrow \frac{-\sqrt{3}/2}{T} \\
f &\rightarrow (1+\nu) \ln T + \ln t'_0 & a &\rightarrow t'_0 T^{1+\nu} & H &\rightarrow \frac{1+\nu}{t'_0} T^{-2-\nu} \\
t &\rightarrow \frac{t'_0}{2+\nu} T^{2+\nu} & z &\rightarrow \frac{a_0}{t'_0} T^{-1-\nu} & T &\rightarrow \left(\frac{2+\nu}{t'_0} t\right)^{1/(2+\nu)} & T &\rightarrow \left(\frac{t'_0}{a_0} z\right)^{-1/(1+\nu)}
\end{aligned} \tag{7.10}$$

$$\begin{aligned}
a &\rightarrow t'_0 \left(\frac{2+\nu}{t'_0}\right)^{1/\sqrt{3}} t^{1/\sqrt{3}} & z &\rightarrow \frac{a_0}{t'_0} \left(\frac{2+\nu}{t'_0}\right)^{-1/\sqrt{3}} t^{-1/\sqrt{3}} & H &\rightarrow \frac{1+\nu}{2+\nu} t^{-1} \\
t &\rightarrow \left(\frac{a_0}{t'_0}\right)^{\sqrt{3}} \left(\frac{2+\nu}{t'_0}\right)^{-1} z^{-\sqrt{3}} & H &\rightarrow \left(\frac{a_0}{t'_0}\right)^{-\sqrt{3}} \left(\frac{1+\nu}{t'_0} z\right) z^{\sqrt{3}}
\end{aligned} \tag{7.11}$$

Substituting the estimated values for  $t'_0$  and  $a_0$

$$\begin{aligned}
\frac{a}{t_H} &\rightarrow 1.1 T^{1.4} & \frac{t}{t_H} &\rightarrow 0.47 T^{2.4} \\
\frac{a}{t_H} &\rightarrow 1.7 \left(\frac{t}{t_H}\right)^{.58} & z &\rightarrow 0.86 \left(\frac{t}{t_H}\right)^{-.58} \\
\frac{t}{t_H} &\rightarrow 0.77 z^{-1.7} & \frac{H}{H_0} &\rightarrow 0.75 z^{1.7}
\end{aligned} \tag{7.12}$$

### 7.4 The limit $t \rightarrow t_{\max}$

In the limit  $T \rightarrow \frac{\pi}{2}$

$$\begin{aligned}
f_T &\rightarrow \frac{\nu}{\frac{\pi}{2}-T} & v_T &\rightarrow \frac{-\sqrt{3}/2}{\frac{\pi}{2}-T} & f &\rightarrow -\nu \ln \left(\frac{\pi}{2}-T\right) + \ln t''_0 \\
a &\rightarrow t''_0 \left(\frac{\pi}{2}-T\right)^{-\nu} & t &\rightarrow t_{\max} - \frac{t''_0}{1-\nu} \left(\frac{\pi}{2}-T\right)^{1-\nu} \\
a &\rightarrow t''_0 \left[ (1-\nu) \left(\frac{t_{\max}-t}{t''_0}\right) \right]^{-1/\sqrt{3}}
\end{aligned} \tag{7.13}$$

### 7.5 Table of parameters for selected $z$ values

|                      | $z$     | $H/H_0$        | $q$   | $w$   | $\Omega$ |
|----------------------|---------|----------------|-------|-------|----------|
| $z \gg 1$            | $\gg 1$ | $0.75 z^{1.7}$ | 0.73  | 0.16  | 1.0      |
|                      | 1000.   | 120000.        | 0.73  | 0.16  | 1.0      |
|                      | 100.    | 2200.          | 0.73  | 0.15  | 1.0      |
|                      | 10.     | 48.            | 0.74  | 0.15  | 1.0      |
| $T = \frac{1}{2}T_0$ | 1.7     | 4.1            | 0.74  | 0.079 | 1.2      |
|                      | 1.0     | 2.4            | 0.69  | 0.021 | 1.3      |
| $q = 0$              | 0.18    | 1.1            | 0.00  | -0.33 | 1.5      |
| $t = t_0$            | 0.00    | 1.0            | -0.60 | -0.61 | 1.5      |

## 7.6 Plot the cosmological parameters

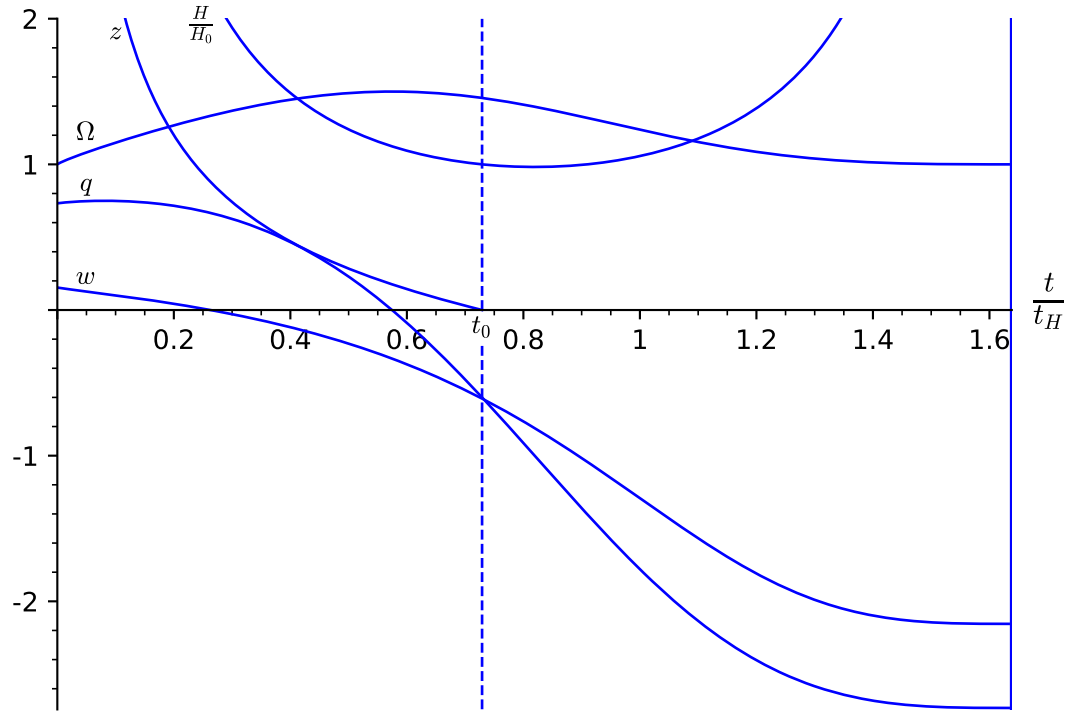

## 7.7 Plot the conformal diagram

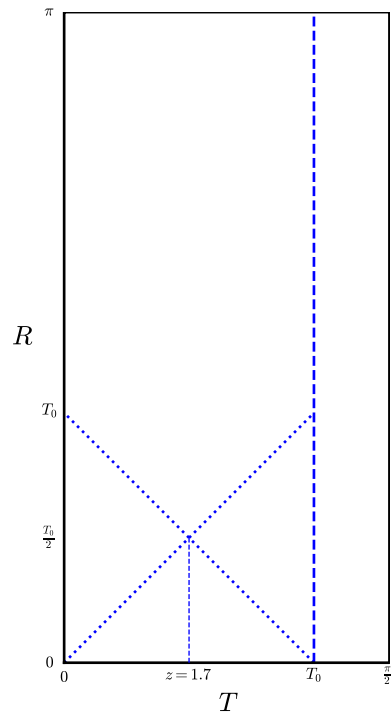

## 8 Analysis of the real-time ode continued

### 8.1 Real-time phase portrait [SNB I-1]

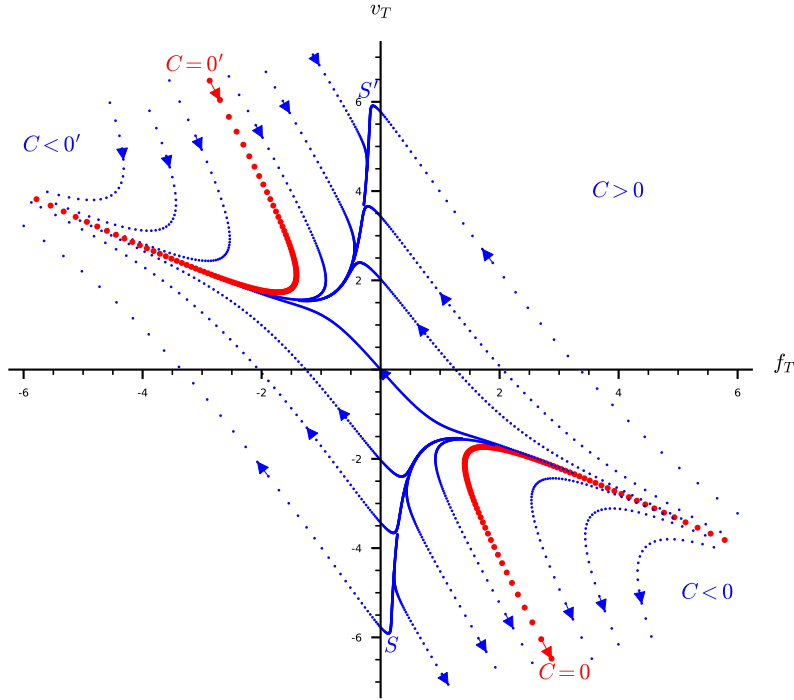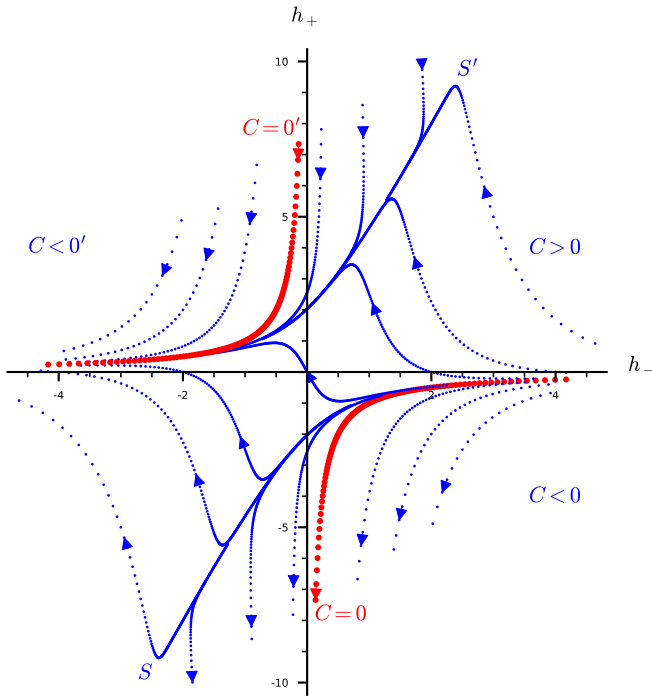

## 8.2 Asymptotic behavior of the $C \neq 0$ solutions

Three asymptotic regions:

1.  $h_+ \rightarrow \pm\infty, \quad |h_-| \leq |h_+|^{1-\epsilon}$
2.  $h_- \rightarrow \pm\infty, \quad |h_+| \leq |h_-|^{1-\epsilon}$
3.  $h_+, h_- \rightarrow \pm\infty, \quad |h_-| \sim |h_+|$

In region 1 we can approximate in the ode (6.3)

$$\begin{aligned} \partial_T h_+ &\rightarrow -h_+^2 & h_+ &\rightarrow \frac{1}{T} & T &\rightarrow 0^\pm \\ f_T &\rightarrow -\frac{\sqrt{3}}{2}\beta_- h_+ \rightarrow \frac{-\nu}{T} & a^2 &\rightarrow a_1^2(T^2)^{-\nu} & h_+ h_- &= -1 + Ca^2 \rightarrow Ca_1^2(T^2)^{-\nu} \\ h_- &\rightarrow Ca_1^2(T^2)^{-\nu} T \rightarrow 0 \end{aligned} \quad (8.1)$$

In region 2

$$\begin{aligned} \partial_T h_- &\rightarrow -h_-^2 & h_- &\rightarrow \frac{1}{T} & T &\rightarrow 0^\pm \\ f_T &\rightarrow \frac{\sqrt{3}}{2}\beta_+ h_- \rightarrow \frac{1+\nu}{T} & a^2 &\rightarrow a_2^2(T^2)^{1+\nu} & h_+ h_- &= -1 + Ca^2 \rightarrow -1 + Ca_2^2(T^2)^{1+\nu} \\ h_+ &\rightarrow -T \rightarrow 0 \\ \partial_T h_+ &\rightarrow -1 - T^2 + \lambda_+ Ca_2^2(T^2)^{1+\nu} + O(T^3) \\ h_+ &\rightarrow -T - \frac{1}{3}T^3 + Ca_2^2(T^2)^{1+\nu}T + O(T^4) \end{aligned} \quad (8.2)$$

In region 3 the only asymptotic trajectories are  $f_T \rightarrow 0, v_T \rightarrow \pm\infty$ . The ode (3.4) is approximated

$$\begin{aligned} \partial_T f_T &= -2(f_T v_T + 1) & \partial_T v_T &= 4f_T v_T + 3 \\ f_T v_T + 1 &\rightarrow 0 & \partial_T v_T &\rightarrow -1 \\ v_T &\rightarrow -T & f_T &\rightarrow \frac{1}{T} & T &\rightarrow \pm\infty \end{aligned} \quad (8.3)$$

In summary, there are three reflection pairs of asymptotic trajectories,

1.  $T \rightarrow 0^\pm \quad h_+ \rightarrow \frac{1}{T} \quad h_- \rightarrow Ca_1^2(T^2)^{-\nu}T$
2.  $T \rightarrow 0^\pm \quad h_- \rightarrow \frac{1}{T} \quad h_+ \rightarrow -T - \frac{1}{3}T^3 + Ca_2^2(T^2)^{1+\nu}T$
3.  $T \rightarrow \pm\infty \quad f_T \rightarrow \frac{1}{T} \quad v_T \rightarrow -T$

Every trajectory asymptotes as type 1 or type 2. Except for the separatrix  $S$  and its reflection  $S'$  every trajectory asymptotes at both ends as type 1 or type 2.  $S$  and  $S'$  each asymptote at one end as type 2.

## 8.3 Non-analyticity of $C \neq 0$ solutions

Try to analytically continue to imaginary time, replacing  $T \rightarrow e^{-i\theta}\tau$  with  $\theta$  ranging from 0 to  $\pi/2$ ,  $f_T \rightarrow e^{i\theta}f_\tau, v_T \rightarrow e^{i\theta}v_\tau, h_\pm \rightarrow e^{i\theta}h_{E\pm}$ . The type 1 and 2 asymptotic behaviors

become

$$\begin{aligned} 1. \quad \tau \rightarrow 0^\pm \quad h_{E+} &\rightarrow \frac{1}{\tau} \quad h_{E-} \rightarrow e^{(2\nu-2)i\theta} C a_1^2 (\tau^2)^{-\nu} \tau \\ 2. \quad \tau \rightarrow 0^\pm \quad h_{E-} &\rightarrow \frac{1}{\tau} \quad h_{E+} \rightarrow \tau - \frac{1}{3} \tau^3 + e^{-(2\nu+4)i\theta} C a_2^2 (T^2)^{1+\eta} T \end{aligned} \quad (8.5)$$

At  $\theta = \pi/2$  this is

$$\begin{aligned} 1. \quad \tau \rightarrow 0^\pm \quad h_{E+} &\rightarrow \frac{1}{\tau} \quad h_{E-} \rightarrow -e^{\nu i\pi} C a_1^2 (\tau^2)^{-\nu} \tau \\ 2. \quad \tau \rightarrow 0^\pm \quad h_{E-} &\rightarrow \frac{1}{\tau} \quad h_{E+} \rightarrow \tau - \frac{1}{3} \tau^3 + e^{-\nu i\pi} C a_2^2 (T^2)^{1+\eta} T \end{aligned} \quad (8.6)$$

but  $h_{E\pm} = f_\tau + \beta_\pm v_\tau$  should be real. So none of the  $C \neq 0$  real-time solutions can be analytic continuations of euclidean signature solutions.

#### 8.4 Asymptotic behavior of the separatrices $S, S'$ [SNB I-1]

The other ends of the separatrices  $S, S'$  have type 3 asymptotic behavior. They have expansions at large  $T$

$$T \rightarrow \pm\infty \quad f_T = \sum_{m=0} f_m T^{-2m-1} \quad v_T = -T + \sum_{m'=0} v_{m'} T^{-2m'-1} \quad f_0 = 1 \quad (8.7)$$

The coefficients  $f_m, v_{m'}$  are determined recursively by the ode (3.4). For  $m \geq 0$

$$\begin{aligned} v_m &= -2f_m + \frac{1}{2m+1} \sum_{m'+m''=m} f_{m'} f_{m''} \\ f_{m+1} &= -\frac{1}{2}(2m+1)f_m + \sum_{m'+m''=m} f_{m'} (f_{m''} + v_{m''}) \end{aligned} \quad (8.8)$$

Numerical calculation for large  $m$  gives

$$\begin{aligned} \frac{-f_m}{f_{m-1}}, \quad \frac{-v_m}{v_{m-1}} &\rightarrow e^{0.5/m} m \\ (-1)^m f_m &\rightarrow 0.22 m^{1/2} m! \quad (-1)^{m+1} v_m \rightarrow 0.44 m^{1/2} m! \end{aligned} \quad (8.9)$$

so the expansions (8.7) are not convergent.

#### 8.5 Numerical calculation of the invariant $c_S$ [SNB I-2]

Calculate

$$\partial_T h_- = -1 - h_-^2 + \lambda_- (h_+ h_- + 1) = -2\nu(1 + h_- f_T) \quad (8.10)$$

Re-write using  $f_T = \partial_T a/a$  and  $2\nu(1 + \nu) = 1$

$$(1 + \nu) \partial_T h_- + h_- \frac{\partial_T a}{a} + 1 = 0 \quad (8.11)$$

Away from  $h_- = 0$  this is

$$\partial_T [(h_-^2)^{1+\nu} a^2] + \frac{2}{h_-} [(h_-^2)^{1+\nu} a^2] = 0 \quad (8.12)$$

For the trajectories that behave as  $h_- \sim T^{-1}$  for  $T \rightarrow 0$  define

$$s = \int_0^T \frac{2 dT'}{h_-(T')} \quad (8.13)$$

so

$$\partial_T [(h_-^2)^{1+\nu} a^2 e^s] = 0 \quad (8.14)$$

so we can define a numerical invariant of the trajectory

$$c = Ca^2 (h_-^2)^{1+\nu} e^s = (h_+ h_- + 1) (h_-^2)^{1+\nu} e^s \quad \partial_T c = 0 \quad (8.15)$$

In the limit  $T \rightarrow 0$

$$c = \lim_{T \rightarrow 0} (h_+ h_- + 1) (h_-^2)^{1+\nu} \quad (8.16)$$

The separatrix  $S$  is one such trajectory. Its invariant  $c_S$  is calculated numerically:

1. Use the large  $T$  expansions (8.7) to get a point on  $S$  at large  $T$ .
2. Numerically integrate the ode backwards to get a point on  $S$  with  $h_- \gg 1$ .
3. Calculate  $s$  as a double expansion  $s(x, y)$

$$x = \frac{1}{h_-^2} \quad y = \frac{h_+ h_- + 1}{h_-^2} = x + \frac{h_+}{h_-} \quad (8.17)$$

Substitute  $s$  in (8.15) to get  $c_S$ .

Calculate

$$\begin{aligned} \partial_T h_- &= -1 - h_-^2 + \lambda_- (h_+ h_- + 1) \\ &= -1 - x^{-1} + x^{-1} \lambda_- y \\ \partial_T h_+ &= -1 - h_+^2 + \lambda_+ (h_+ h_- + 1) = -1 - (h_- y - h_-^{-1})^2 + \lambda_+ x^{-1} y \\ &= -1 - x^{-1} y^2 + 2y - x + \lambda_+ x^{-1} y \end{aligned} \quad (8.18)$$

$$h_- \partial_T x = \frac{-2}{h_-^2} \partial_T h_- = -2x [-1 - x^{-1} + x^{-1} \lambda_- y] = 2(1 + x - \lambda_- y)$$

$$\partial_T (h_- y) = \partial_T (h_+ + h_-^{-1})$$

$$\begin{aligned} h_- \partial_T y &= \partial_T (h_- y) - y \partial_T h_- = \partial_T (h_+ + h_-^{-1}) - y \partial_T h_- = \partial_T h_+ - (x + y) \partial_T h_- \\ &= (-1 - x^{-1} y^2 + 2y - x + \lambda_+ x^{-1} y) - (x + y)(-1 - x^{-1} + x^{-1} \lambda_- y) \\ &= (1 + \lambda_+) x^{-1} y + (3 - \lambda_-) y - (1 + \lambda_-) x^{-1} y^2 \\ &= 2x^{-1} y [(2 + \nu) + (1 + \nu)x - (1 - \nu)y] \end{aligned} \quad (8.19)$$

so

$$\begin{aligned} \frac{1}{2} h_- \partial_T x &= \partial_s x = 1 + x - \lambda_- y \\ \frac{1}{2} h_- \partial_T y &= \partial_s y = x^{-1} y [(2 + \nu) + (1 + \nu)x - (1 - \nu)y] \end{aligned} \quad (8.20)$$

$(2 + \nu)\lambda_- = (1 - \nu)$  so

$$\begin{aligned} xy^{-1} \partial_s y - (2 + \nu) \partial_s x &= -x \\ \partial_s [\ln y - (2 + \nu) \ln x + s] &= 0 \\ yx^{-2-\nu} e^s &= c \quad \partial_s c = 0 \end{aligned} \quad (8.21)$$

Consider  $e^s$  as a function  $e^s(x, y)$  defined by

$$e^s(0, 0) = 1 \quad e^s = \partial_s e^s = \partial_s x \partial_x e^s + \partial_s y \partial_y e^s \quad (8.22)$$

which is

$$x e^s = (1 + x - \lambda_- y) x \partial_x e^s + [(2 + \nu) + (1 + \nu)x - (1 - \nu)y] y \partial_y e^s \quad (8.23)$$

At  $y = 0$  the solution is

$$e^s(x, 0) = 1 + x \quad (8.24)$$

Expand around  $x = y = 0$

$$e^s = \sum_{j,k \geq 0} \mathcal{S}_{j,k} x^j y^k \quad (8.25)$$

$$\begin{aligned} x \sum_{j,k \geq 0} \mathcal{S}_{j,k} x^j y^k &= (1 - \lambda_- y + x) \sum_{j,k \geq 0} \mathcal{S}_{j,k} j x^j y^k \\ &\quad + [(2 + \nu) - (1 - \nu)y + (1 + \nu)x] \sum_{j,k \geq 0} \mathcal{S}_{j,k} k x^j y^k \end{aligned} \quad (8.26)$$

$$\begin{aligned} \mathcal{S}_{j-1,k} &= j \mathcal{S}_{j,k} - \lambda_- j \mathcal{S}_{j,k-1} + (j-1) \mathcal{S}_{j-1,k} \\ &\quad + (2 + \nu) k \mathcal{S}_{j,k} - (1 - \nu)(k-1) \mathcal{S}_{j,k-1} + (1 + \nu) k \mathcal{S}_{j-1,k} \end{aligned}$$

So we get a recursion formula

$$[j + (2 + \nu)k] \mathcal{S}_{j,k} = [2 - j - (1 + \nu)k] \mathcal{S}_{j-1,k} + [\lambda_- j + (1 - \nu)(k-1)] \mathcal{S}_{j,k-1} \quad (8.27)$$

For  $j = 0$

$$\begin{aligned} (2 + \nu)k \mathcal{S}_{0,k} &= (1 - \nu)(k-1) \mathcal{S}_{0,k-1} \\ \mathcal{S}_{0,k} &= 0 \quad k \geq 1 \end{aligned} \quad (8.28)$$

so the recursion can start from

$$\mathcal{S}_{0,0} = 1 \quad \mathcal{S}_{1,0} = 1 \quad \mathcal{S}_{j,0} = 0 \quad j \geq 2 \quad \mathcal{S}_{0,k} = 0 \quad k \geq 1 \quad (8.29)$$

The expansion might be cut off at  $O(x^N)$  according to

$$\begin{aligned} y &= O(x^{2+\nu}) \quad x^j y^k = O(x^{j+k(2+\nu)}) = O(x^N) \quad j + k(2 + \nu) \leq N \\ j &\leq N \quad k \leq N/(2 + \nu) \end{aligned} \quad (8.30)$$

## 9 Euclidean signature phase portrait [SNB I-3]

The phase portrait of the euclidean signature ode (2.4) is shown for completeness. It is not used in the paper.

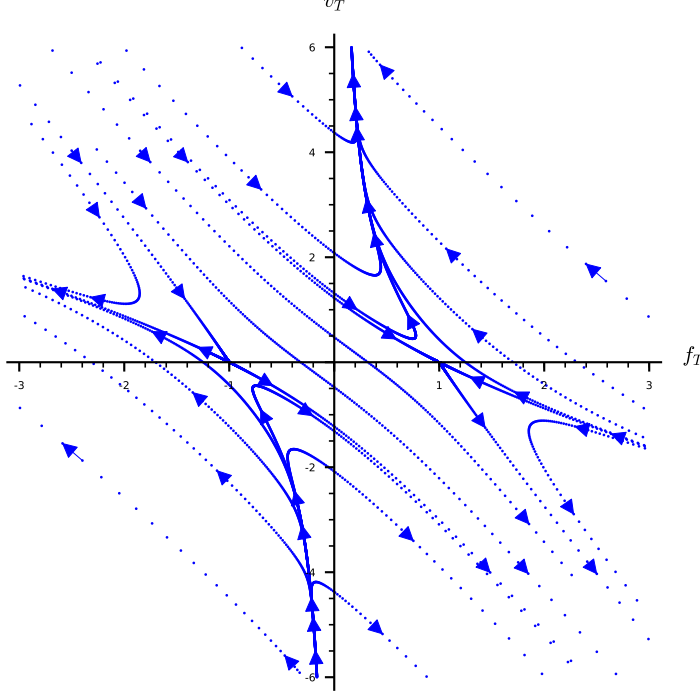

The ode

$$\partial_\tau f_\tau = -2f_\tau v_\tau - 2f_\tau^2 + 2 \quad \partial_\tau v_\tau = 4f_\tau v_\tau + 3f_\tau^2 - 3 \quad (9.1)$$

is regarded as a dynamical system. A solution is a trajectory in the  $f_\tau, v_\tau$  plane parametrized by  $\tau$ . The ode is invariant under the time-reflection symmetry

$$\tau \rightarrow -\tau \quad (f_\tau, v_\tau) \rightarrow (-f_\tau, -v_\tau) \quad (9.2)$$

There are two fixed points, at  $(1, 0)$  and at its reflection  $(-1, 0)$ . The linearized ode at  $(1, 0)$  is

$$\partial_\tau \begin{pmatrix} \Delta f_\tau + \Delta v_\tau \\ 3\Delta f_\tau + \Delta v_\tau \end{pmatrix} = \begin{pmatrix} 2 & 0 \\ 0 & -2 \end{pmatrix} \begin{pmatrix} \Delta f_\tau + \Delta v_\tau \\ 3\Delta f_\tau + \Delta v_\tau \end{pmatrix} \quad (9.3)$$

so the fixed point has an unstable manifold tangent to  $\Delta v_\tau = -3\Delta f_\tau$  and a stable manifold tangent to  $\Delta v_\tau = -\Delta f_\tau$ .

The analytic continuation of the  $C = 0$  solution (6.7) from  $T$  to  $\tau = iT$  is

$$f_\tau = -\frac{\cosh 2\tau + \sqrt{3}}{\sinh 2\tau} \quad v_\tau = \frac{\sqrt{3}}{\sinh 2\tau} \quad (9.4)$$

In the phase portrait this is the union of two trajectories. The portion  $-\infty \leq \tau < 0$  is the unstable trajectory leaving the fixed point  $(1, 0)$  going into the lower-right quadrant. The portion  $0 < \tau \leq \infty$  is the time-reflection, the stable trajectory of the fixed point  $(-1, 0)$  entering from the upper-left quadrant. The two trajectories are joined at the point at  $\infty$  in the  $(f_\tau, v_\tau)$  plane at  $\tau = 0$

$$(f_\tau, v_\tau) \rightarrow \left( -\frac{1 + \sqrt{3}}{2\tau}, \frac{\sqrt{3}}{2\tau} \right) \quad \tau \rightarrow 0^\pm \quad (9.5)$$

The phase portrait is calculated using numerical integration from initial conditions at large  $f_\tau$ . The trajectories which reach large  $f_\tau$  are given asymptotically by expansions around  $\tau = 0$

$$f_\tau = \tau^{-1} \sum_{m,n=0} \beta^m (\tau^2)^{m\alpha/2} \tau^{2n} \mathbf{f}_{m,n} \quad v_\tau = \tau^{-1} \sum_{m,n=0} \beta^m (\tau^2)^{m\alpha/2} \tau^{2n} \mathbf{v}_{m,n} \quad (9.6)$$

where  $\alpha$  is a positive real number to be determined and  $\beta$  is a real number which parametrizes the trajectory and ranges over some interval around 0. The coefficients  $\mathbf{f}_{m,n}$  and  $\mathbf{v}_{m,n}$  are given by recursion relations obtained by substituting in the ode. For  $(m,n) = (0,0)$

$$\begin{aligned} -\mathbf{f}_{0,0} &= \mathbf{f}_{0,0} (-2\mathbf{v}_{0,0} - 2\mathbf{f}_{0,0}) \\ -\mathbf{v}_{0,0} &= \mathbf{f}_{0,0} (4\mathbf{v}_{0,0} + 3\mathbf{f}_{0,0}) \end{aligned} \quad \begin{pmatrix} \mathbf{f}_{0,0} \\ \mathbf{v}_{0,0} \end{pmatrix} = \begin{pmatrix} \frac{1}{2} + \epsilon \frac{\sqrt{3}}{2} \\ -\epsilon \frac{\sqrt{3}}{2} \end{pmatrix} \quad \epsilon = \pm 1 \quad (9.7)$$

Then the recursion relation for  $(m,n) \neq (0,0)$  is

$$\begin{aligned} A_{m,n} \begin{pmatrix} \mathbf{f}_{m,n} \\ \mathbf{v}_{m,n} \end{pmatrix} &= \delta_{m,0} \delta_{n,1} \begin{pmatrix} 2 \\ -3 \end{pmatrix} + \begin{pmatrix} -2 & -2 \\ 3 & 4 \end{pmatrix} \sum_{\substack{m'+m''=m \\ n'+n''=n \\ \neq (0,0),(m,n)}} \mathbf{f}_{m',n'} \begin{pmatrix} \mathbf{f}_{m'',n''} \\ \mathbf{v}_{m'',n''} \end{pmatrix} \\ A_{m,n} &= \begin{pmatrix} \alpha m + 2n - 1 + 2\mathbf{v}_{0,0} + 4\mathbf{f}_{0,0} & 2\mathbf{f}_{0,0} \\ -4\mathbf{v}_{0,0} - 6\mathbf{f}_{0,0} & \alpha m + 2n - 1 - 4\mathbf{f}_{0,0} \end{pmatrix} \\ \det A_{m,n} &= (\alpha m + 2n + 1)(\alpha m + 2n - 3 - \epsilon\sqrt{3}) \end{aligned} \quad (9.8)$$

The case  $(m,n) = (1,0)$  requires

$$\det A_{1,0} = 0 \quad \alpha = 3 + \epsilon\sqrt{3} \quad \begin{pmatrix} \mathbf{f}_{1,0} \\ \mathbf{v}_{1,0} \end{pmatrix} = \begin{pmatrix} 1 \\ -1 - \epsilon\sqrt{3} \end{pmatrix} \quad (9.9)$$

Then  $\det A_{m,n} \neq 0$  for  $(m,n) \neq (1,0)$  so the recursion relation determines all the remaining coefficients.

## 10 $v_\mu = \partial_\mu \chi \iff \chi$ is the dilaton field

If  $v_\mu = \partial_\mu \chi$ , the fixed point equation is

$$R_{\mu\nu} = 2\nabla_\mu \nabla_\nu \chi \quad (10.1)$$

and  $\chi$  satisfies

$$\nabla_\mu \nabla^\mu \chi + 2\nabla_\mu \chi \nabla^\mu \chi - C' = 0 \quad (10.2)$$

These are the equations of motion of the dilaton action

$$S = \int d^d x \sqrt{g} e^{2\chi} (-R - 4\nabla_\mu \chi \nabla^\mu \chi - 2C') \quad (10.3)$$

So if  $v_\mu = \partial_\mu \chi$  then  $\chi$  is the dilaton field. But  $v^\mu$  is not necessarily a gradient in general.

To derive the dilaton equations of motion, first vary  $\chi \rightarrow \chi + \delta\chi$

$$\begin{aligned} \delta S &= \int d^d x \sqrt{g} e^{2\chi} [2\delta\chi(-R - 4\nabla_\mu \chi \nabla^\mu \chi - 2C') - 8\nabla_\mu \chi \nabla^\mu \delta\chi] \\ &= \int d^d x \sqrt{g} e^{2\chi} \delta\chi [-2R - 8\nabla_\mu \chi \nabla^\mu \chi - 4C' + 8e^{-2\chi} \nabla^\mu (e^{2\chi} \nabla_\mu \chi)] \\ &= \int d^d x \sqrt{g} e^{2\chi} \delta\chi [-2R - 8\nabla_\mu \chi \nabla^\mu \chi - 4C' + 4e^{-2\chi} (\nabla^\mu \nabla_\mu) e^{2\chi}] \end{aligned} \quad (10.4)$$

Vary  $g_{\mu\nu} \rightarrow g_{\mu\nu} + \delta g_{\mu\nu}$  using

$$\begin{aligned}\delta R_{\mu\nu} &= \frac{1}{2} [\nabla_\sigma \nabla_\mu \delta g_\nu^\sigma + \nabla_\sigma \nabla_\nu \delta g_\mu^\sigma - \nabla^\sigma \nabla_\sigma \delta g_{\mu\nu} - \nabla_\mu \nabla_\nu \delta g_\sigma^\sigma] \\ g^{\mu\nu} \delta R_{\mu\nu} &= \nabla_\mu \nabla_\nu \delta g^{\mu\nu} - g_{\mu\nu} \nabla^\sigma \nabla_\sigma \delta g^{\mu\nu}\end{aligned}\quad (10.5)$$

$$\begin{aligned}\delta S &= \int d^d x \sqrt{g} e^{2\chi} \left[ \frac{1}{2} \delta g^{\mu\nu} g_{\mu\nu} (-R - 4\nabla_\sigma \chi \nabla^\sigma \chi - 2C') - \delta g^{\mu\nu} (-R_{\mu\nu} - 4\nabla_\mu \chi \nabla_\nu \chi) - g^{\mu\nu} \delta R_{\mu\nu} \right] \\ &= \int d^d x \sqrt{g} e^{2\chi} \left[ \frac{1}{2} \delta g^{\mu\nu} g_{\mu\nu} (-R - 4\nabla_\sigma \chi \nabla^\sigma \chi - 2C') - \delta g^{\mu\nu} (-R_{\mu\nu} - 4\nabla_\mu \chi \nabla_\nu \chi) \right. \\ &\quad \left. + (-\nabla_\mu \nabla_\nu \delta g^{\mu\nu} + g_{\mu\nu} \nabla^\sigma \nabla_\sigma \delta g^{\mu\nu}) \right] \\ &= \int d^d x \sqrt{g} e^{2\chi} \delta g^{\mu\nu} \left[ R_{\mu\nu} + 4\nabla_\mu \chi \nabla_\nu \chi - \frac{1}{2} g_{\mu\nu} (R + 4\nabla_\sigma \chi \nabla^\sigma \chi + 2C') \right. \\ &\quad \left. + e^{-2\chi} (-\nabla_\mu \nabla_\nu + g_{\mu\nu} \nabla^\sigma \nabla_\sigma) e^{2\chi} \right]\end{aligned}\quad (10.6)$$

So the equations of motion are

$$\begin{aligned}0 &= R + 4\nabla_\mu \chi \nabla^\mu \chi + 2C' - 2e^{-2\chi} (\nabla^\mu \nabla_\mu) e^{2\chi} \\ 0 &= R_{\mu\nu} + 4\nabla_\mu \chi \nabla_\nu \chi - \frac{1}{2} g_{\mu\nu} (R + 4\nabla_\sigma \chi \nabla^\sigma \chi + 2C') \\ &\quad + e^{-2\chi} (-\nabla_\mu \nabla_\nu + g_{\mu\nu} \nabla^\sigma \nabla_\sigma) e^{2\chi}\end{aligned}\quad (10.7)$$

Substituting the first equation of motion in the second, the second becomes

$$0 = R_{\mu\nu} - 2\nabla_\mu \nabla_\nu \chi \quad (10.8)$$

so

$$R = 2\nabla^\mu \nabla_\mu \chi \quad (10.9)$$

Substituting for  $R$ , the first equation of motion becomes

$$0 = \nabla_\mu \nabla^\mu \chi + 2\nabla_\mu \chi \nabla^\mu \chi - C' \quad (10.10)$$

So the dilaton equations of motion are

$$R_{\mu\nu} = 2\nabla_\mu \nabla_\nu \chi \quad \nabla^\mu \nabla_\mu \chi + 2\nabla^\mu \chi \nabla_\mu \chi - C' = 0 \quad (10.11)$$
